# Supplementary material for: OneCast: Structured Decomposition and Modular Generation for Cross-Domain Time Series Forecasting
Source: arXiv:2510.24028 source file (2025-11-03)
Supplement: Supplementary file 1 [file appendix_H.tex]

\begin{table*}[hb]
\centering
\caption{Multivariate time series forecasting full results evaluated by MAE $\downarrow$.}
\setlength{\tabcolsep}{2.5pt}
\resizebox{\textwidth}{!}{
\begin{tabular}{@{}cc|cccc|ccccccc@{}}
\toprule
\multicolumn{2}{c|}{\multirow{2}{*}{\textbf{Method}}} & \multicolumn{4}{c|}{\textbf{Models Trained Across-Domain}} & \multicolumn{6}{c}{\textbf{Models Trained In-Domain}} \\ \cmidrule(l){3-13} 
\multicolumn{2}{c|}{} & OneCast & UniTime & TOTEM & TimesFM & PatchTST & FEDformer & Autoformer & DLinear & MICN & FILM \\ \midrule \midrule

\multicolumn{1}{c|}{\multirow{4}{*}{\rotatebox{90}{Traffic}}} & 24 & \underline{0.312} & 0.357 & 0.328 & 0.348 & 0.358 & 0.357 & 0.368 & 0.384 &\textbf{0.298} & 0.372 \\
\multicolumn{1}{c|}{} & 48 & \underline{0.339} & 0.367 & 0.349 & 0.345 & 0.383 & 0.360 & 0.379 & 0.397 & \textbf{0.300} & 0.377 \\
\multicolumn{1}{c|}{} & 96 & \underline{0.332} & 0.362 & 0.355 & 0.353 & 0.372 & 0.356 & 0.370 & 0.401 & \textbf{0.312} & 0.362 \\
\multicolumn{1}{c|}{} & 192 & \underline{0.338} & 0.366 & 0.368 & 0.352 & 0.359 & 0.378 & 0.391 & 0.388 &\textbf{0.317} & 0.368 \\ \midrule

\multicolumn{1}{c|}{\multirow{4}{*}{\rotatebox{90}{Weather}}} & 24 & \textbf{0.151} & 0.166 & 0.183 & 0.158 & \underline{0.153} & 0.255 & 0.255 & 0.170 & 0.174 & 0.185 \\
\multicolumn{1}{c|}{} & 48 & \textbf{0.194} & 0.201 & 0.227 & 0.211 & \underline{0.200} & 0.298 & 0.306 & 0.222 & 0.225 & 0.207 \\
\multicolumn{1}{c|}{} & 96 & \underline{0.236} & 0.238 & 0.239 & 0.236 & \textbf{0.234} & 0.320 & 0.325 & 0.253 & 0.249 & 0.237 \\
\multicolumn{1}{c|}{} & 192 & 0.273 & \underline{0.265} & 0.280 & 0.273 & \textbf{0.263} & 0.342 & 0.350 & 0.298 & 0.289 & 0.271 \\ \midrule

\multicolumn{1}{c|}{\multirow{4}{*}{\rotatebox{90}{CzeLan}}} & 24 & \textbf{0.219} & 0.255 & 0.248 & 0.233 & \underline{0.224} & 0.268 & 0.424 & 0.315 & 0.299 & 0.335 \\
\multicolumn{1}{c|}{} & 48 & 0.274 & \underline{0.273} & 0.281 & 0.288 & \textbf{0.270} & 0.336 & 0.548 & 0.384 & 0.341 & 0.360 \\
\multicolumn{1}{c|}{} & 96 & \textbf{0.265} & 0.292 & 0.299 & 0.292 & \underline{0.275} & 0.324 & 0.493 & 0.359 & 0.376 & 0.313 \\
\multicolumn{1}{c|}{} & 192 & \textbf{0.285} & 0.328 & 0.319 & 0.302 & \underline{0.294} & 0.363 & 0.598 & 0.425 & 0.432 & 0.341 \\ \midrule

\multicolumn{1}{c|}{\multirow{4}{*}{\rotatebox{90}{ETTh2}}} & 24 & \textbf{0.264} & 0.285 & 0.307 & 0.297 & \textbf{0.264} & 0.324 & 0.359 & \underline{0.270} & 0.308 & 0.288 \\
\multicolumn{1}{c|}{} & 48 & \textbf{0.313} & \underline{0.315} & 0.343 & 0.320 & 0.329 & 0.355 & 0.373 & 0.318 & 0.343 & 0.323 \\ 
\multicolumn{1}{c|}{} & 96 & 0.358 & 0.352 & 0.383 &\underline{0.349} & \textbf{0.341} & 0.394 & 0.408 & 0.386 & 0.407 & 0.364 \\
\multicolumn{1}{c|}{} & 192 & 0.408 & \underline{0.400} & 0.429 & \underline{0.400} & \textbf{0.391} & 0.442 & 0.451 & 0.475 & 0.489 & 0.420 \\ \midrule

\multicolumn{1}{c|}{\multirow{4}{*}{\rotatebox{90}{ETTm2}}} & 24 & \textbf{0.202} & 0.225 & 0.230 & 0.225 & 0.210 & 0.239 & 0.257 & 0.210 & \underline{0.208} & 0.210 \\
\multicolumn{1}{c|}{} & 48 & 0.247 & 0.249 & 0.254 & 0.251 & \textbf{0.233} & 0.263 & 0.273 & 0.247 & \underline{0.240} & 0.243 \\
\multicolumn{1}{c|}{} & 96 & 0.291 & 0.271 & 0.278 & 0.284 & \textbf{0.261} & 0.287 & 0.310 & 0.292 & 0.282 & \underline{0.266} \\
\multicolumn{1}{c|}{} & 192 & 0.318 & 0.310 & 0.340 & 0.348 & \textbf{0.303} & 0.331 & 0.339 & 0.361 & 0.360 & \underline{0.306} \\ \midrule

\multicolumn{1}{c|}{\multirow{4}{*}{\rotatebox{90}{FRED-MD}}} & 24 & \textbf{0.872} & 1.182 & 1.304 & \underline{0.888} & 1.100 & 1.636 & 1.714 & 1.621 & 2.044 & 1.478 \\
\multicolumn{1}{c|}{} & 36 & \textbf{0.940} & 1.484 & 1.482 & \underline{1.111} & 1.447 & 1.883 & 1.953 & 1.905 & 1.965 & 1.882 \\
\multicolumn{1}{c|}{} & 48 & \textbf{1.460} & 1.722 & 1.695 & \underline{1.543} & 1.747 & 2.138 & 2.195 & 2.220 & 2.652 & 2.087 \\
\multicolumn{1}{c|}{} & 60 & \textbf{1.808} & 2.213 & \underline{1.834} & 1.851 & 2.112 & 2.436 & 2.489 & 2.531 & 3.107 & 2.413 \\ 
\midrule

\multicolumn{1}{c|}{\multirow{4}{*}{\rotatebox{90}{NYSE}}} & 24 & 0.369 & \underline{0.335} & 0.349 & 0.342 & 0.362 & \textbf{0.330} & 0.466 & 0.573 & 0.584 & 0.448 \\
\multicolumn{1}{c|}{} & 36 & \textbf{0.353} & 0.428 & 0.445 & \underline{0.410} & 0.418 & 0.447 & 0.508 & 0.702 & 0.573 & 0.512 \\
\multicolumn{1}{c|}{} & 48 & \textbf{0.427} & 0.491 & 0.505 & \underline{0.459} & 0.532 & 0.550 & 0.605 & 0.802 & 0.796 & 0.583 \\
\multicolumn{1}{c|}{} & 60 & \textbf{0.517} & 0.613 & 0.597 & \underline{0.535} & 0.614 & 0.626 & 0.714 & 0.938 & 0.988 & 0.720 \\ \midrule

\multicolumn{1}{c|}{\multirow{4}{*}{\rotatebox{90}{Covid-19}}} & 24 & \textbf{0.043} & 0.046 & 0.073 & \underline{0.044} & 0.047 & 0.187 & 0.276 & 0.426 & 0.521 & 0.070 \\
\multicolumn{1}{c|}{} & 36 & \textbf{0.053} &\underline{0.054} & 0.093 & 0.055 & 0.058 & 0.198 & 0.256 & 0.463 & 0.520 & 0.064 \\
\multicolumn{1}{c|}{} & 48 & 0.067 & \textbf{0.063} & 0.091 & 0.069 & \underline{0.066} & 0.217 & 0.253 & 0.381 & 0.783 & 0.072 \\
\multicolumn{1}{c|}{} & 60 & \underline{0.075} & \textbf{0.073} & 0.093 & 0.078 & \underline{0.075} & 0.233 & 0.277 & 0.551 & 0.927 & 0.083 \\ \midrule

\multicolumn{1}{c|}{\multirow{4}{*}{\rotatebox{90}{Wike2000}}} & 24 & \textbf{1.048} & 1.118 & 1.208 & 1.163 & \underline{1.093} & 3.839 & 3.912 & 1.277 & 1.451 & 1.408 \\
\multicolumn{1}{c|}{} & 36 & \textbf{1.150} & \underline{1.217} & 1.341 & 1.379 & 1.271 & 3.245 & 3.302 & 1.362 & 1.363 & 1.533 \\
\multicolumn{1}{c|}{} & 48 & \textbf{1.223} & \underline{1.299} & 1.356 & 1.347 & 1.314 & 3.092 & 3.076 & 1.439 & 1.565 & 1.617 \\
\multicolumn{1}{c|}{} & 60 & \textbf{1.282} & 1.341 & 1.360 & 1.353 & \underline{1.321} & 2.938 & 2.921 & 1.514 & 1.706 & 1.672 \\ 
\midrule
\multicolumn{2}{c|}{$1^{\text{st}}$ Counts} & 21 & 2 & 0 & 0 & 9 & 1 & 0 & 0 & 4 & 0 &  \\ \bottomrule\bottomrule
\end{tabular}
}
\label{tab:mae}
\end{table*}
