# Supplementary material for: OneCast: Structured Decomposition and Modular Generation for Cross-Domain Time Series Forecasting
Source: arXiv:2510.24028 source file (2025-11-03)
Supplement: Supplementary file 2 [file related_work.tex]

\section{Related Work}

\textbf{Time series forecasting.} Time series forecasting is a critical technique in real world. Traditional methods such as ARIMA \cite{hyndman2008forecasting} are primarily based on statistics, relying on statistic assumptions (linearity, stationarity, ect.). These methods offer strong interpretability but struggle to handle complex nonlinear relationships. With the rise of machine learning, data-driven forecasting approaches such as tree-based XGBoost \cite{zhang2021time} and LightGBM \cite{ke2017lightgbm}, have been proposed, significantly improving the ability to model nonlinear relationships in time series data. 

As deep learning advanced, many deep learning-based time series methods have been developed, which can capture temporal and cross-dimensional dependencies in multivariate time series. For example, Transformer-based architectures like Autoformer \cite{wu2021autoformer} and Fedformer \cite{zhou2022fedformer} approach the problem from temporal and frequency domain perspectives, respectively, using deep decomposition architectures to iteratively extract more predictable components for future data modeling. Beyond these, other architectures also exhibit promising performance in time series forecasting, such as CNN-based TimesNet \cite{wu2022timesnet} and MICN \cite{wang2023micn}, MLP-based DLinear \cite{zeng2023transformers}, and LM-based methods \cite{liu2024time,jin2023time} etc.

\textbf{Cross-domain modeling. } The core challenge in cross-domain modeling centers on developing a unified representation to represent data across domains. A critical issue therein is mitigating channel count inconsistency across domains. Existing cross-domain methods are categorized into two types based on input representation: continuous and discrete.

Continuous methods (e.g., UniTime \cite{liu2024unitime}, TimesFM \cite{das2024decoder}) segment sequences into patches and adopt patch embedding spaces as unified input representation spaces. Discrete methods, by contrast, employ discrete symbols as intermediaries to encode sequences into unified discrete symbol representations. For example, Chronos \cite{ansari2024chronos} and LLMTime \cite{gruver2023large} leverage quantiles of the overall distribution to map each numerical point in sequences to discrete IDs via a binning strategy, thus enabling cross-domain representation unification but overlooking semantic-level encoding and modeling.  On this basis, PromptCast \cite{xue2023promptcast} takes a different approach by directly representing numerical sequences as text and leveraging the powerful understanding and reasoning capabilities of language models for forecasting. While this encoding method demonstrates strong potential, it neglects the sparsity characteristics inherent in sequence data, making it challenging to effectively model long-term forecasting tasks.
