# Supplementary material for: OneCast: Structured Decomposition and Modular Generation for Cross-Domain Time Series Forecasting
Source: arXiv:2510.24028 source file (2025-11-03)
Supplement: Supplementary file 4 [file appendix_I.tex]

\section{Limitations}

Despite significant progress in cross-domain sequence prediction, OneCast is constrained by the discrete diffusion paradigm, which prevents it from extending to arbitrary-length sequence outputs as autoregressive generation does. Besides, we do not consider the issue of severe data imbalance between different domains, which may limit the ability to generalize to diverse datasets.
